# Supplementary material for: Robust spectral clustering with rank statistics
Source: arXiv:2408.10136 source file (2024-12-19)
Supplement: Supplementary file 1 [file jrc_RSCR_sec_appendix.tex]

% appendix with additional proof details.
